# Supplementary material for: Emergence of Disordered Hyperuniformity in Melts of Linear Diblock Copolymers
Source: arXiv:2312.08541 source file (2024-03-22)
Supplement: Supplementary file 1 [file si_micelle_prl.pdf]

# Supplemental Material: Emergence of Disordered Hyperuniformity in Melts of Linear Diblock Copolymers

Duyu Chen,[1,*] Michael A. Klatt,[2,3,4] and Glenn H. Fredrickson[1,5,†]

[1] *Materials Research Laboratory, University of California, Santa Barbara, California 93106, United States*
[2] *Institut für KI Sicherheit, Deutsches Zentrum für Luft- und Raumfahrt (DLR), Wilhelm-Runge-Str. 10, 89081 Ulm, Germany*
[3] *Institut für Materialphysik im Weltraum, Deutsches Zentrum für Luft- und Raumfahrt (DLR), 51170 Köln, Germany*
[4] *Department of Physics, Ludwig-Maximilians-Universität, Schellingstr. 4, 80799 Munich, Germany*
[5] *Department of Chemical Engineering, University of California, Santa Barbara, California 93106, United States*

## S1. REPRESENTATIVE CONFIGURATION AND ENSEMBLE-AVERAGED STRUCTURE FACTOR FOR INITIAL SPHERE CENTERS

In Fig. S1(a) we show a representative configuration with $N_s = 2000$ points for point patterns that correspond to the local energy minima of the Quantizer energy, which appears to be disordered. As mentioned in the main text, we use these point patterns as the initial positions for the micelle centers in our SCFT simulations. The ensemble-averaged $S(k)$ at unit density of these point patterns is shown in Fig. S1(b), which is effectively zero (on the order of $10^{-3}$) for a range of small $k$ for both system sizes, indicating that the point patterns that correspond to the local energy minima of the Quantizer energy are (effectively) stealthy hyperuniform. These results are consistent with those in previous work [1].

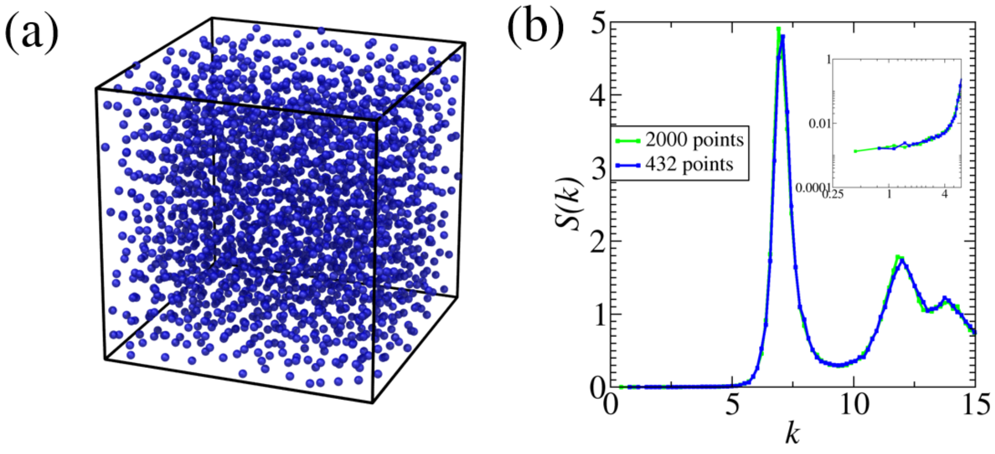


FIG. 1: (Color online) Visualization of an example with $N_s = 2000$ points (a) and the ensemble-averaged structure factor $S(k)$ (b) of the point patterns of the inherent structures (i.e., local energy minima) of the "Quantizer energy" at unit number density (averaged over 10 configurations).

## S2. SINGLE-CHAIN PARTITION FUNCTION AND SPECIES DENSITY FIELD

For the incompressible melts of AB linear diblock copolymers, the single-chain partition function $Q[w_A, w_B]$ [2] is given by

$$Q[w_A, w_B] = \frac{1}{V} \int_V d\mathbf{r}\; q(\mathbf{r}, N; [w_A, w_B]), \tag{1}$$

where $q(\mathbf{r}, N; [w_A, w_B])$ is the forward chain propagator, and $N$ is the degree of polymerization. As mentioned in the main text, in this work we employ the discrete Gaussian chain model, and the forward chain propagator

$q(\mathbf{r}, j; [w_A, w_B])$ is given by

$$q(\mathbf{r}, j+1; [w_A, w_B]) = \begin{cases} e^{-w_A(\mathbf{r})} \int d\mathbf{r}' \phi(\mathbf{r}-\mathbf{r}') q(\mathbf{r}', j; [w_A, w_B]) & j = 1, \cdots, N_A - 1 \\ e^{-w_B(\mathbf{r})} \int d\mathbf{r}' \phi(\mathbf{r}-\mathbf{r}') q(\mathbf{r}', j; [w_A, w_B]) & j = N_A, \cdots, N - 1 \end{cases} \tag{2}$$

where $N_A$, $N_B$ are the degrees of polymerization for the A and B blocks, respectively, $N = N_A + N_B$, the Gaussian-type linker function $\phi(r)$ is given by $\phi(r) = (\frac{3}{2\pi b^2})^{3/2} \exp(-\frac{3r^2}{2b^2})$, and $b$ is the statistical segment length (in this work we assume $b$ is the same for A and B monomers). The initial condition of $q(\mathbf{r}, j; [w_A, w_B])$ is given by

$$q(\mathbf{r}, 1; [w_A, w_B]) = e^{-w_A(\mathbf{r})}. \tag{3}$$

Similarly, one can define the backward chain propagator $q_C(\mathbf{r}, j; [w_A, w_B])$ as

$$q_C(\mathbf{r}, j+1; [w_A, w_B]) = \begin{cases} e^{-w_B(\mathbf{r})} \int d\mathbf{r}' \phi(\mathbf{r}-\mathbf{r}') q_C(\mathbf{r}', j; [w_A, w_B]) & j = 1, \cdots, N_B - 1 \\ e^{-w_A(\mathbf{r})} \int d\mathbf{r}' \phi(\mathbf{r}-\mathbf{r}') q_C(\mathbf{r}', j; [w_A, w_B]) & j = N_B, \cdots, N - 1 \end{cases} \tag{4}$$

The initial condition of $q_C(\mathbf{r}, j; [w_A, w_B])$ is given by

$$q_C(\mathbf{r}, 1; [w_A, w_B]) = e^{-w_B(\mathbf{r})}. \tag{5}$$

Then, the density field $\rho_A(\mathbf{r}; [w_A, w_B]$ can be computed as

$$\rho_A(\mathbf{r}; [w_A, w_B] = \frac{n e^{w_A(\mathbf{r})}}{VQ[w_A, w_B]} \sum_{j=1}^{N_A} q(\mathbf{r}, j; [w_A, w_B]) q_C(\mathbf{r}, N+1-j; [w_A, w_B]) \tag{6}$$

## S3. SCFT SIMULATION DETAILS

The self-consistent field equations [2] are solved numerically on a uniform spatial collocation mesh with periodic boundary conditions, and the field updates are performed using the semi-implicit Seidel (SIS) scheme [2]. We find that a spatial resolution of $128 \times 128 \times 128$ is sufficient to resolve the mesostructures of the disordered hyperuniform micelles (a larger resolution of $192 \times 192 \times 192$ leads to a change in free energy only on the order of $10^{-7} k_B T$ per chain), which has a comparable spatial resolution per sphere to that used in the recent theory work [3] for liquid-like packings. A spatial resolution of $64 \times 64 \times 64$ is used for the unit-cell SCFT simulations of the BCC sphere mesophase. The simulations are considered converged when the field and stress errors fell below $10^{-5}$ and $10^{-4}$, respectively, which are deemed sufficient for the thermodynamic properties of interest.

## S4. NUMERICAL CALCULATION OF STRUCTURE FACTOR

Upon spatial discretization, for $\mathbf{k} \neq \mathbf{0}$, $S(\mathbf{k})$ can be computed as

$$S(\mathbf{k}) = \frac{1}{V} \tilde{m}^2(\mathbf{k}) |\tilde{\mathcal{J}}(\mathbf{k})|^2, \tag{7}$$

where the indicator function of a discretization unit (or voxel) $\tilde{m}(\mathbf{k})$ is given by

$$\tilde{m}(\mathbf{k}) = \tilde{m}_x(k_x) \tilde{m}_y(k_y) \tilde{m}_z(k_z), \tag{8}$$

and the generalized collective coordinate [4] $\tilde{\mathcal{J}}(\mathbf{k})$ is given by

$$\tilde{\mathcal{J}}(\mathbf{k}) = \sum_{\mathbf{r}} \exp(-i\mathbf{k} \cdot \mathbf{r}) [\rho_A(\mathbf{r}) - f_A]. \tag{9}$$

Here the component $\tilde{m}_i(k_i)$ of the voxel indicator function is given by

$$\tilde{m}_i(k_i) = \begin{cases} \frac{\sin(k_i l_i/2)}{k_i/2} & k_i \neq 0 \\ l_i & k_i = 0 \end{cases} \tag{10}$$

where $l_i$ is the side length of a voxel along the $i$-th direction. For a cubic box subject to periodic boundary conditions, the component of a wavevector $k_i$ can only take the values of $k_i = 2\pi n_i/L$, where $L$ is the side length of the cubic box, and $n_i$ is an integer, and one can compute $\tilde{\mathcal{J}}(\mathbf{k})$ efficiently using the standard fast Fourier transform algorithm. Then $S(\mathbf{k})$ is angular-averaged and binned according to the magnitude of $k = |\mathbf{k}|$ to obtain $S(k)$.

* correspondence sent to: duyu@alumni.princeton.edu
† correspondence sent to: ghf@mrl.ucsb.edu

[1] M. A. Klatt, J. Lovrić, D. Chen, S. C. Kapfer, F. M. Schaller, P. W. A. Schönhöfer, B. S. Gardiner, A. Smith, G. E. Schröder-Turk, and S. Torquato, Nat. Commun. **10**, 1 (2019).
[2] G. H. Fredrickson, *The equilibrium theory of inhomogeneous polymers*, 134 (Oxford University Press: Oxford, 2006).
[3] K. D. Dorfman and Z.-G. Wang, ACS Macro Lett. **12**, 980 (2023).
[4] D. Chen and S. Torquato, Acta Mater. **142**, 152 (2018).
